# Supplementary material for: Hard Thermal Loop -- theory and applications
Source: arXiv:2404.08734 source file (2024-09-19)
Supplement: Supplementary file 1 [file appendix_ph.tex]

\subsection*{Thermal Rate of Real Photon Production}
\label{phot_appendix}
Let us now consider real photon emission from a system in thermal equilibrium. We consider a transition from an initial state $i$ to final state $f$ and a photon
with momentum $P\equiv (E=p_0, \bm{\vec p})$ and polarisation $\epsilon^\mu(P)$. The transition rate is given as~\cite{Gale:1990pn}
\be
R_{fi} =\frac{\left | S_{fi} \right |^2}{\tau V} \, . \label{prate0}
\ee
where $V$ is the volume of the system and $\tau$ is the observation time.
The matrix element can be written as
\bea
S_{fi}&=& \left.\left\langle f;\, \gamma\right. \right | \int d^4x J_\mu(x)A^\mu(x)\left. \left | i \right \rangle \right. \label{prate1}
\eea
where $J_\mu(x)$ is the electromagnetic current of the strongly interacting particles which produces the photon and $A^\mu(x)$ is the free photon field and given as
\be
A^\mu(x)=\frac{\epsilon^\mu}{\sqrt{2EV}} \left(e^{iP.x}+ e^{-iP.x}\right ) \, , \label{prate2}
\ee
and the photon polarisation sum is given as
\be
\sum_{\textrm{polarisation}} \epsilon^\mu\epsilon^\nu=-g^{\mn} \, .\label{prate3}
\ee
Since the photon escapes without re-interacting, the matrix element can be  factorised as
\be
\left.\left\langle f;\, \gamma\right. \right | J_\mu(x)A^\mu(x)\left. \left | i \right \rangle \right.  =  \left.\left\langle f\right. \right | J_\mu(x)\left. \left | i \right \rangle \right.  \, 
\left.\left\langle  \gamma\right. \right | A^\mu(x)\left. \left | 0\right \rangle \right.  \, . \label{prate4}
\ee
Using \eqref{prate2} and \eqref{prate4} in \eqref{prate1} one can write
\be
S_{fi}= \frac{\epsilon^\mu}{\sqrt{2EV}} \int d^4x  \left(e^{iP.x}+ e^{-iP.x}\right ) \left.\left\langle f\right. \right | J_\mu(x)\left. \left | i \right \rangle \right. \, . \label{prate5}
\ee
Now, inserting \eqref{prate5} and \eqref{prate3} in \eqref{prate0} along with translational invariance, one gets
\be
R_{fi} = - \frac{g^{\mn}}{EV}  \int d^4x  \left(e^{iP.x}+ e^{-iP.x}\right )  \left.\left\langle f\right. \right | J_\mu(x)\left. \left | i \right \rangle \right. 
 \left.\left\langle i\right. \right | J_\nu(x)\left. \left | f \right \rangle \right. \, .\label{prate6}
\ee
Applying translational invariance again
\be
 \left.\left\langle f\right. \right | J_\mu(x)\left. \left | i \right \rangle \right. = e^{i\left(K_i-K_f\right)\cdot x}\, \left.\left\langle f\right. \right | J_\mu(0)\left. \left | i \right \rangle \right.\, , \label{prate7}
\ee
and using it in \eqref{prate6}, one can write
\bea
R_{fi} &=& -  \frac{g^{\mn}}{EV} \, \left(2\pi\right )^4 \, \Big[\delta\left(K_i-P-K_f\right)+\delta\left(K_i+P-K_f\right) \Big]\,
\left.\left\langle f\right. \right | J_\mu(0)\left. \left | i \right \rangle \right. \left.\left\langle i\right. \right | J_\nu(0)\left. \left | f \right \rangle \right.\, , \label{prate8}
\eea
where the first $\delta$-function corresponds to photon emission where as that of second one corresponds to absorption. Since we are interested in emission of photon, the second
$\delta$-function can be neglected.

Now we average the initial state  with the Boltzmann weight  $e^{-\beta {\cal K}_i}/{\cal Z}(\beta)$, where ${\cal Z}(\beta)=\sum_j e^{-\beta {\cal K}_j}$ with ${\cal K}=H-\mu N$, and sum over final states. The the thermal photon multiplicity per unit volume can be written from \eqref{prate8} as
\be
\frac{dR}{d^4x} = -  \frac{g^{\mn}}{EV}  \frac{Vd^3\bm{\vec p}}{(2\pi)^3} \frac{1}{{\cal Z}(\beta)} \sum_i e^{-\beta {\cal K}_i} \sum_f \left(2\pi\right )^4 \delta\left(K_i-K_f- P\right)
\left.\left\langle f\right. \right | J_\mu(0)\left. \left | i \right \rangle \right. \left.\left\langle i\right. \right | J_\nu(0)\left. \left | f \right \rangle \right.\, . \label{prate9}
\ee
Now one can define current-current correlation functions along with some identities~\cite{Fradkin} as
\be
G^\pm_{\mn}(P) = \pm \frac{1}{{\cal Z}(\beta)} \sum_{if} e^{-\beta {\cal K}_i}  \left(2\pi\right )^4 \delta\left(K_i-K_f\pm P\right)
\left.\left\langle f\right. \right | J_\mu(0)\left. \left | i \right \rangle \right. \left.\left\langle i\right. \right | J_\nu(0)\left. \left | f \right \rangle \right.\, , \label{prate10}
\ee
where $G^+_{\mn}(P)$ and $G^-_{\mn}(P)$ related by microscopic detailed balance corresponding to absorption and emission as
\be
G^+_{\mn}(P) =-e^{\beta E} G^-_{\mn}(P) \, . \label{prate11}
\ee
The retarded and temperature correlation functions are given as~\cite{Gale:1990pn}
\begin{subequations}
\begin{align}
G^R_{\mn}(P) &=\int\limits_{-\infty}^{\infty}\frac{dE'}{2\pi}\,\, \frac{\rho^n_{\mn}(E',\bm{\vec p}) }{E'-E-i\epsilon} \, , \label{prate11a} \\
G^T_{\mn}(P) &=\int\limits_{-\infty}^{\infty}\frac{dE'}{2\pi} \,\, \frac{\rho^n_{\mn}(E',\bm{\vec p}) }{E'-i\om_n} \, ;\,\,\,\, \,\,\,\,\,\,\,\,  \om_n=2n\pi T \label{prate11b} 
\end{align}
\end{subequations}
are defined through  the same  spectral function as
\be
\rho^n_{\mn} = G^+_{\mn} + G^-_{\mn} = -\left(e^{\beta E}-1\right )  G^-_{\mn} \, . \label{prate12}
\ee
Now, $G^R_{\mn}(P) = {\cal P}^R_{\mn}(P)$ is retarded improper photon self-energy defined through the relation
\be
D^{R,\alpha\beta}= D^{R,\alpha\beta}_0 + D^{R,\alpha\mu}_0  {\cal P}^R_{\mn}  D^{R,\nu\beta}_0 \, . \label{prate13}
\ee
and one  gets
\be
\rho^n_{\mn}(P) =-2 {\textrm{Im}}  {\cal P}^R_{\mn} (P) \, . \label{prate14}
\ee
Combining \eqref{prate12} and \eqref{prate14} one obtains the fluctuation-dissipation theorem~\cite{forster,Callen:1951vq,Kubo:1957mj}
\be
 G^-_{\mn} (P)=  - \frac{\rho^n_{\mn}(P) }{\left(e^{\beta E}-1\right ) } =   \frac{2}{\left(e^{\beta E}-1\right ) } {\textrm{Im}}  {\cal P}^R_{\mn} (P) \, . \label{prate15}
\ee
In order ${\cal O}(e^2)$, the improper self-energy $ {\cal P}_{\mn} (P)$ becomes equal to proper self-energy $\Pi_{\mn}(P)$ of photon which is defined as
\be
D^{\alpha\beta}= D^{\alpha\beta}_0 + D^{\alpha\mu}_0  {\Pi}_{\mn}  D^{\nu\beta} \, . \label{prate16}
\ee
Combining \eqref{prate10} and \eqref{prate15} then inserting in \eqref{prate9} one obtains the real photon emission rate from a thermal medium as
\bea
E\frac{dR}{d^4x d^3 \bm{\vec p}}&=& \frac{2  g^{\mn}}{(2\pi)^3} \, \frac{1}{\left(e^{\beta E}-1\right ) }\, \textrm{Im}\Big[\Pi_{\mn}(E,\bm{\vec  p})\Big] \, \nn
&=& \frac{2 }{(2\pi)^3} \, n_B(E) \, \textrm{Im}\Big[\Pi^{\mu}_{\mu}(E,\bm{\vec  p})\Big]   , \label{prate17}
\eea
which agrees with \eqref{ph3}.
